# Supplementary material for: Scalable Sampling for High Utility Patterns
Source: arXiv:2410.22964 source file (2024-10-30)
Supplement: Supplementary file 1 [file appendix.tex]

%\section{Theoretical analysis of the method}
%\label{sub:analysis}
%\input{tex/analysis.tex}

%\section{\myalgoOff: On-disk Quantitative Pattern Sampling}
%\myalgoOff emerges as a vital solution for HUP sampling, particularly in scenarios where the complete database surpasses the constraints of available main memory. In the realm of exploratory data analysis, the challenge of efficiently drawing high utility patterns from large databases has been a persistent issue. \myalgoOff addresses this challenge by offering an on-disk alternative, ensuring that the limitations of limited-size RAM are circumvented without compromising the algorithm effectiveness. Its significance becomes especially pronounced when dealing with vast datasets, where in-memory methods such \myalgo struggle to accommodate the sheer volume of information. By providing a robust on-disk approach, \myalgoOff facilitates the efficient sampling of patterns, enabling users to extract valuable insights from extensive qDBs without the constraints imposed by limited RAM resources.

\section{Additional experiments}
%%%%%%%%%%%%%%%%%%%%%%%%%%%%%%%%%%%%%%%%%%%%%%%%%%%%%%%%%%%%%%%%%%%%%%%%%%%%%%%%%%%%%%%%%%%%%%
\subsection{Representativeness study with \myalgo}
\label{sec:QualitativeAnalysis}
%!TEX root = ../QPlus.tex

In this section, we study the representativeness of the sampled patterns and check if the patterns drawn by \myalgo follow the same distribution that those drawn by \HAISampler in high average utility patterns sampling. Let the maximum length constraint be $\maxLen=10$ and the number of patterns to draw be $1,000$. We consider the following databases for evaluation:  \retail, \bmsDeux, and \chainstoreFIM. Figure \ref{fig:comparison_quality} gives the distribution of the average utility according the pattern lengths.

\begin{figure}[htp!]
	\centering
	
	\includegraphics[width=.23 \textwidth, keepaspectratio]{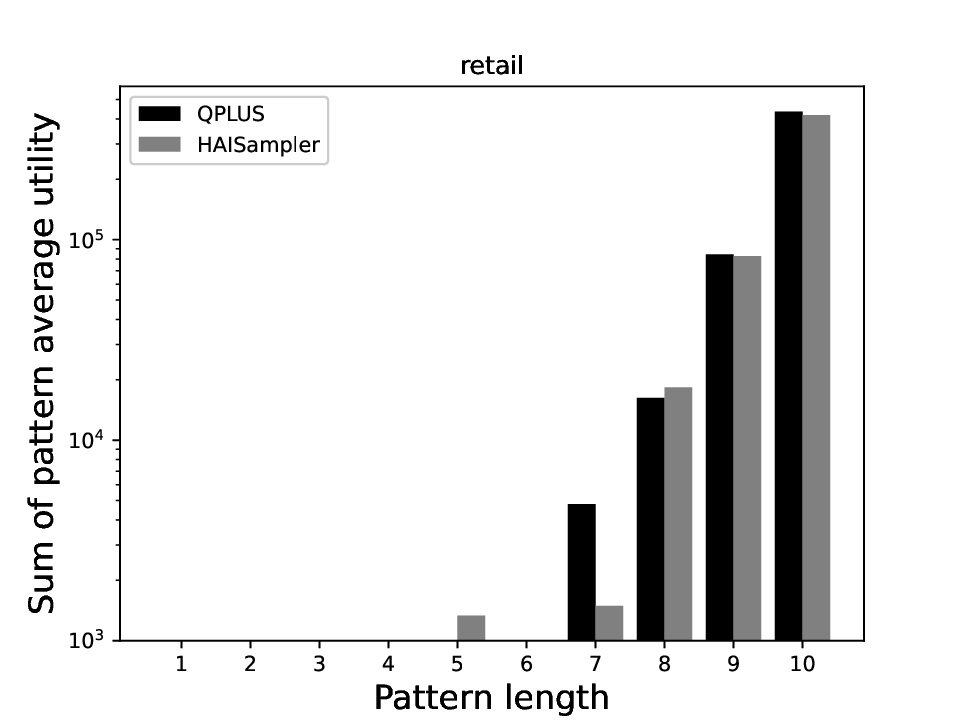}
	\includegraphics[width=.23 \textwidth, keepaspectratio]{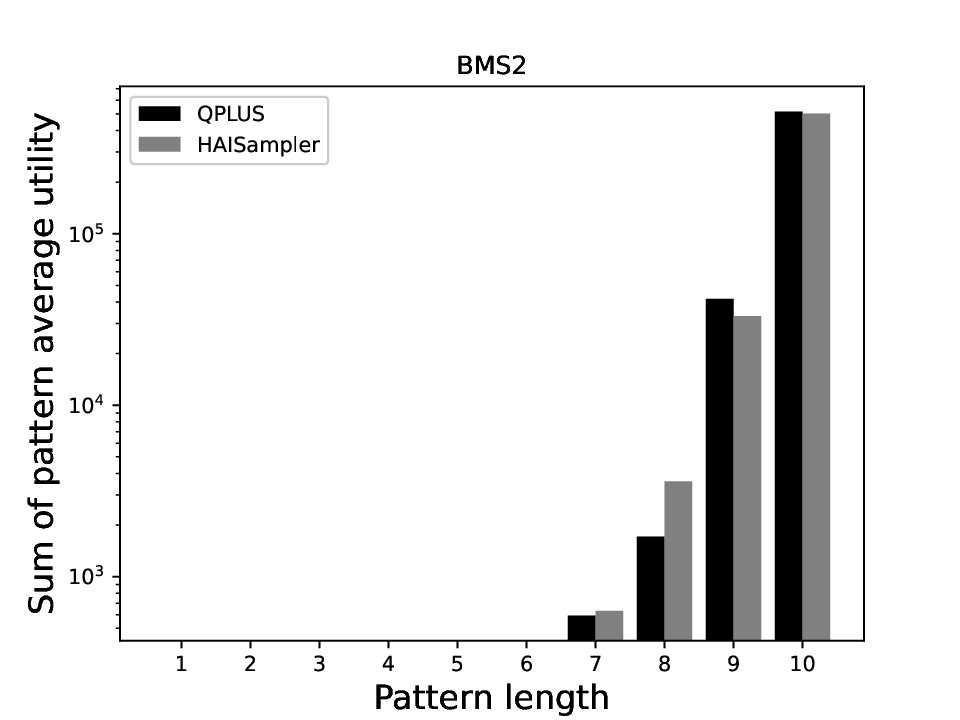}

	\includegraphics[width=.23 \textwidth, keepaspectratio]{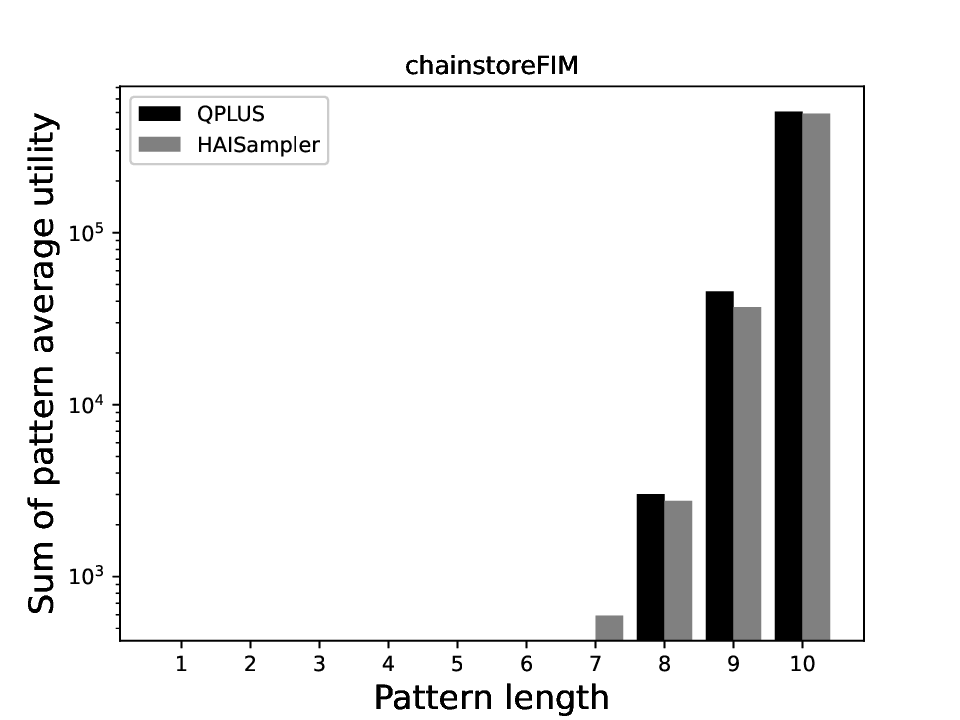}
	\includegraphics[width=.23 \textwidth, keepaspectratio]{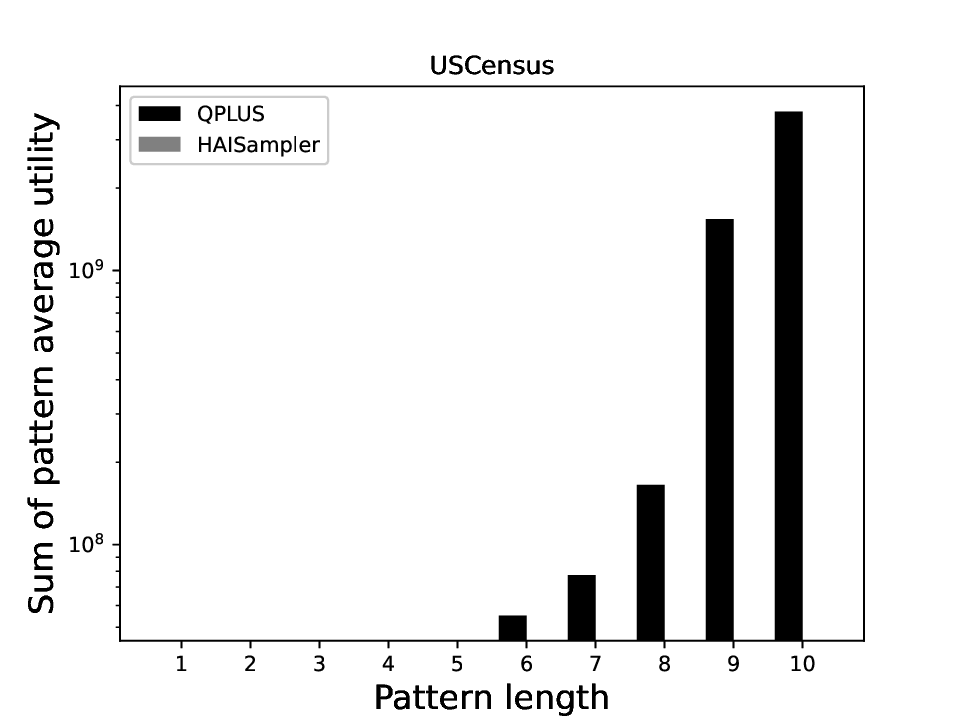}
	
	\caption{Comparing the distribution of 1,000 drawn patterns by \myalgo and \HAISampler }
	\label{fig:comparison_quality}
\end{figure}

%
%Let us now examine whether we have the same distribution as \HAISampler. Figure \ref{fig:comparison_quality} shows the distribution of the sampled patterns according to their lengths. 
Focusing on \myalgo on one hand, we can see that, the drawn patterns have high average utilities with different lengths. Interestingly, the most sampled patterns have very high utility values. 
On the other hand, as we can see that, we have approximately the same distribution in all of the considered quantitative databases which implies that \myalgo and \HAISampler follow the same distribution. Hence, we can conclude that our jumping based on dichotomous random search, Property \ref{prop:dichotomous_random_search}, sounds good.

\subsection{Sub-profile sampling on \DBpedia}
\label{sec:dbpedia}

This section delves into supplementary experimental findings pertaining to the exploration of high utility patterns (HUPs) for sub-profile discovery within extensive knowledge graphs, such as \DBpedia. Building upon the context of our study, we investigate to large-scale knowledge graphs, aiming to unveil insights into the efficiency and performance of \myalgo in this challenging and intricate domain. The experiments confirm the results obtained in \DOREMUS and \BENICULTURALI in the main paper, and show that, the given profile is centered around the class ``dbo:Organisation''\footnote{\url{https://dbpedia.org/ontology/Organisation}, dbo=https://dbpedia.org/ontology/} of \DBpedia, in particular around concepts such as ``dbo:Company'', ``dbo:Place'' and ``dbo:Location''.

\subsection{Response time for interactive sub-profile discovery} To integrate \myalgo into the \KGSUMVIZ\footnote{\url{https://github.com/DTTProfiler/DTTProfiler}} tool for sub-profile discovery when the user interacts with the profile via the tool, we need a fast processing and a fast drawing. This response time depends on the characteristics of the corresponding qDB and in particular, the longest transaction (node of the graph with highest incoming/outgoing degree), the average transaction size and the number of transactions. With $\maxLen=5$, the processing time for \DOREMUS, \BENICULTURALI and \DBpedia are respectively $0.004$ second, $0.018$ second, and $0.023$ second, while the drawing time per pattern are respectively $0.069$ millisecond, $0.127$ millisecond, and $0.141$ milliseconds. Therefore, it is possible to return a sub-profile of hundreds nodes and thousands links less than $1$ millisecond. However, for a clear visualization in practice, the number of nodes and that of links are not high.

\begin{table}[htp!]
    \begin{tabular}{cc}
        \begin{minipage}{.22\textwidth}
            \centering
            \includegraphics[width=\linewidth, keepaspectratio]{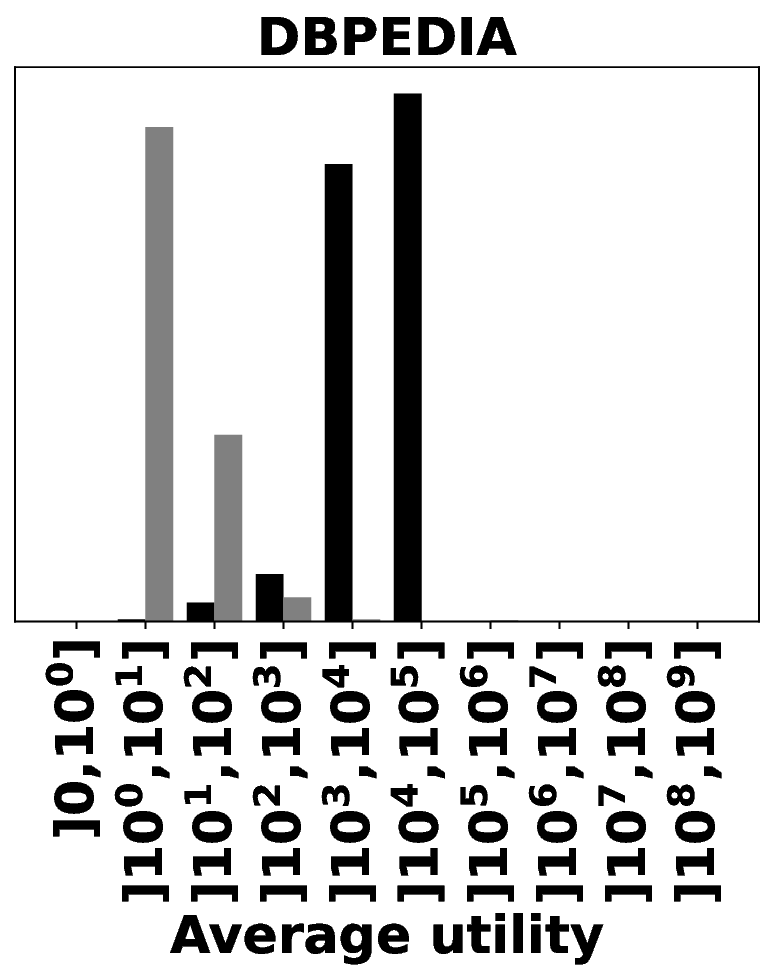}
            \caption{Comparing the representativeness of distinct patterns from 1,000 drawn patterns by \myalgo and Bootstrap }
            \label{fig:comparison_quality_QPLUSvsBootstrap1}
        \end{minipage}
        &
        \begin{minipage}{.25\textwidth}
            \centering
            \includegraphics[width=\linewidth, keepaspectratio]{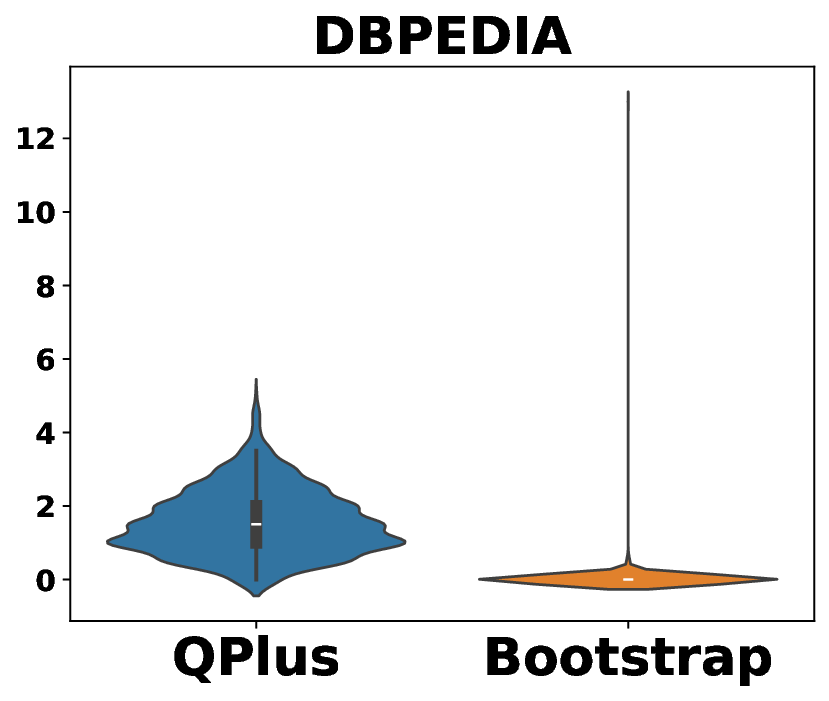}
            \caption{Violin plots with mean and 95\% confidence intervals for the plus-value of \myalgo on Bootstrap}
            \label{fig:plus-values1}
        \end{minipage}
    \end{tabular}
\end{table}

\begin{table}[htp!]
    \begin{tabular}{cc}
        \begin{minipage}{.2\textwidth}
            \centering
            \includegraphics[width=\linewidth, keepaspectratio]{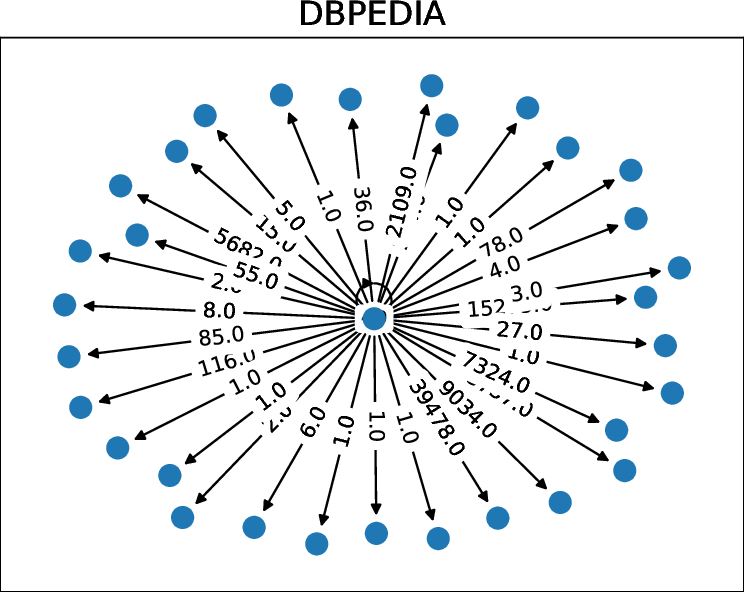}
            \label{fig:viz-subprofile1}
        \end{minipage}
        &
        \begin{minipage}{.2\textwidth}
            \centering
            \includegraphics[width=\linewidth, keepaspectratio]{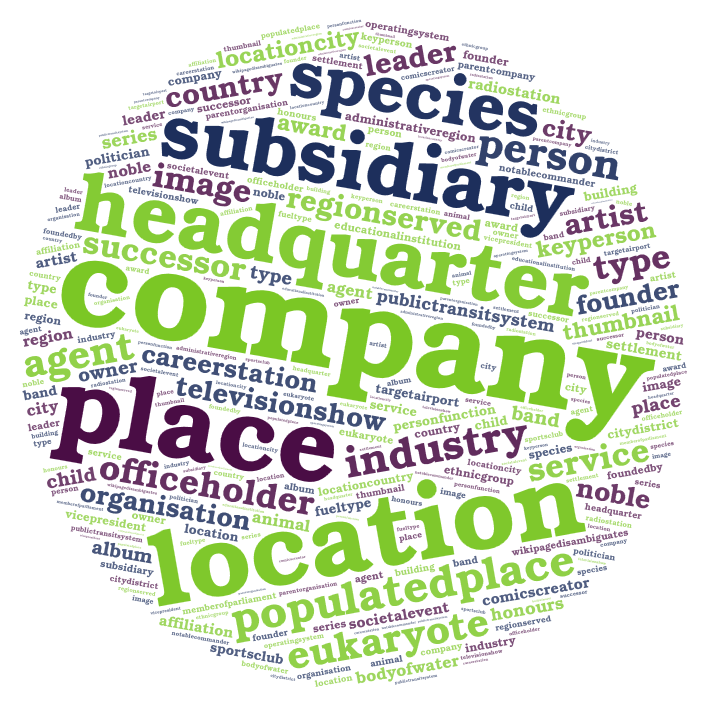}
            \label{fig:viz-subprofile2}
        \end{minipage}
    \end{tabular}
    \caption{Visualizing sub-profiles from 10 patterns of maximal length $\maxLen=5$ drawn by \myalgo}
    \label{tab:my_label1}
\end{table}

\section{Proofs}

\begin{proof}(Property \ref{prop:VUTU_symmetry})
    We know that $\vutu_\trans(\uLen, i) = \binom{i-1}{\uLen-1} \times \vutu_\trans(1, i)$ holds for all $\uLen$ according to Theorem \ref{theo:vutu}. We can derive $\vutu_\trans(i-\uLen+1, i) = \binom{i-1}{i-\uLen+1-1} \times \vutu_\trans(1, i) = \binom{i-1}{i-\uLen} \times \vutu_\trans(1, i)$. Since $\binom{i-1}{\uLen-1} = \binom{i-1}{i-\uLen}$, this property becomes trivial and holds true.
\end{proof}

\begin{proof}(Property \ref{prop:dichotomous_random_search})
This property is somewhat trivial because, after using Bayes' Theorem and Definition \ref{def:probability_item_selection}, it stems from simplifying the intermediate values which do not allow selecting their corresponding item based on their randomly generated variables.
\end{proof}

\begin{sloppypar}
\begin{proof}(Property \ref{prop:soundness})
    Given two positive integers \minLen and \maxLen such that $\minLen \leq \maxLen$, let $Z$ be the normalization constant defined as the sum of the utility of all patterns of the qDB \database under the length constraint. Formally, $Z = \sum_{\pattern \in \lang_{[\minLen..\maxLen]}(\database)} \left( \utility(\pattern, \database) \times f_{[\minLen..\maxLen]}(\uLen) \right)$. Let $\prob_{[\minLen..\maxLen]}(\pattern, \database)$ be the probability to draw pattern \pattern from the set of patterns in \database using algorithm \myalgo under the length constraint. We have $\prob_{[\minLen..\maxLen]}(\pattern, \database)=\sum_{\trans \in \database}\prob(\pattern, \trans) = \sum_{\trans \in \database} \prob(\trans) \prob_{[\minLen..\maxLen]}(\pattern | \trans)$. Based on line 2, we get $\prob(\trans)=\frac{W_{[\minLen..\maxLen]}(\trans)}{Z}$. From the third and fourth lines, we know that $\prob_{[\minLen..\maxLen]}(\pattern | \trans) = \prob(\uLen | \trans) \times \prob(\pattern | \trans \wedge \uLen)$. Line 3 also shows that $\prob(\uLen | \trans) = \frac{\vutu_\trans(\uLen, \card{\trans})\times f_{[\minLen..\maxLen]}(\uLen)}{\sum_{\uLen' = \minLen}^{\maxLen} (\vutu_\trans(\uLen', \card{\trans}) \times f_{[\minLen..\maxLen]}(\uLen'))} = \frac{\vutu_\trans(\uLen, \card{\trans})\times f_{[\minLen..\maxLen]}(\uLen)}{W_{[\minLen..\maxLen]}(\trans)}$.
    We also know from lines 7 and 8 that $\prob(\pattern | \trans \wedge \uLen)=\frac{\utilityTrans(\pattern, \trans)}{\sum_{\pattern' \in \trans \wedge \card{\pattern'} \in [\minLen..\maxLen]} \utilityTrans(\pattern', \trans)}=\frac{\utilityTrans(\pattern, \trans) \times f_{[\minLen..\maxLen]}(\uLen)}{\vutu_\trans(\uLen, \card{\trans}) \times f_{[\minLen..\maxLen]}(\uLen)}$. By substitution, we have 
    $\prob_{[\minLen..\maxLen]}(\pattern, \database)=\sum_{\trans \in \database} (\frac{W_{[\minLen..\maxLen]}(\trans)}{Z} \times \frac{\vutu_\trans(\uLen, \card{\trans})\times f_{[\minLen..\maxLen]}(\uLen)}{W_{[\minLen..\maxLen]}(\trans)} \times \frac{\utilityTrans(\pattern, \trans) \times f_{[\minLen..\maxLen]}(\uLen)}{\vutu_\trans(\uLen, \card{\trans}) \times f_{[\minLen..\maxLen]}(\uLen)})= \sum_{\trans \in \database} \frac{\utilityTrans(\pattern, \trans) \times f_{[\minLen..\maxLen]}(\uLen)}{Z} = \frac{f_{[\minLen..\maxLen]}(\uLen)}{Z} \times (\sum_{\trans \in \database} \utilityTrans(\pattern, \trans))$. Thanks to Definition \ref{def:patternutility}, $\utility(\pattern, \database) = \sum_{\trans \in \database} \utilityTrans(\pattern, \trans)$. Then, we can conclude that $\prob_{[\minLen..\maxLen]}(\pattern, \database) = \frac{f_{[\minLen..\maxLen]}(\uLen)}{Z} \times \utility(\pattern, \database)$, which shows that \pattern is drawn proportionally to its weighted utility and completes this proof.
\end{proof}
\end{sloppypar}

\begin{proof}(Property \ref{prop:pascal})
    By exploiting the symmetric property $\Cnk{i}{j} = \Cnk{i}{i-j}$, we need only to store the ($\floor{\frac{i}{2}}+1$) first values of row $i$, with $i \in [0..n]$. Let $g(i)=\floor{\frac{i}{2}}+1$ for all $i \in [0..n]$. With $n+1$ rows, the total number of combination values that needed to be stored is compute by $G(n)=\sum_{i=0}^{n}g(i)$. First, let us break down the sum into its individual terms: $g(0)=\floor{\frac{0}{2}}+1=0+1=1$; $g(1)=\floor{\frac{1}{2}}+1=0+1=1$; $g(2)=\floor{\frac{2}{2}}+1=1+1=2$; $g(3)=\floor{\frac{3}{2}}+1=1+1=2$; $g(4)=\floor{\frac{4}{2}}+1=2+1=3$; so on ... Notice that, the term $\floor{\frac{i}{2}}+1$ takes on the values 1, 1, 2, 2, 3, 3, ... as $i$ increases. This is because $g(2k+1)=\floor{\frac{2k+1}{2}}+1=\frac{2k}{2}+\floor{\frac{1}{2}} +1=\frac{2k}{2}+1=\floor{\frac{2k}{2}}+1=g(2k)$, for all positive integer $k$. Therefore, we now distinguish two cases.
    
    \noindent Case 1: $n$ is even, i.e, $n = 2\times k$ with $k$ a positive integer. In that case, $\floor{\frac{n}{2}}=\floor{\frac{2\times k}{2}}=\frac{n}{2}$. Then, we have $G(n)= 2 \times (\sum_{j=1}^{\frac{n}{2}}j) + g(n) = 2\times \frac{\frac{n}{2}(\frac{n}{2}+1)}{2} + \frac{n}{2}+1=\frac{n}{2}\times(\frac{n}{2}+1)+ \frac{n}{2}+1=(\frac{n}{2}+1)\times(\frac{n}{2}+1)$. Hence, we got $G(n)=(\frac{n}{2}+1)^2$.
    
    \noindent Case 2: $n$ is odd, i.e, $n-1$ is even, and $g(n)=\floor{\frac{n}{2}}+1=\frac{n-1}{2}+1$. Therefore, we have $G(n)= G(n-1)+g(n)=(\frac{n-1}{2}+1)^2+\frac{n-1}{2}+1=(\frac{n+1}{2})^2+\frac{n+1}{2}=\frac{n+1}{2}(\frac{n+1}{2}+1)=\frac{n+1}{2}\times\frac{n+3}{2}$. Hence, we got $G(n)=(n+1)\times\frac{n+3}{4}$.
    %\noindent Based on these two cases, we can say that Property \ref{prop:pascal} holds.  
\end{proof}
